# Supplementary material for: Architectural Complexity Measures of Recurrent Neural Networks
Source: arXiv:1602.08210 source file (2016-11-12)
Supplement: Supplementary file 1 [file appendix.tex]

%\begin{document}
\onecolumn
\title{Supplementary  Materials: Architectural Complexity Measures of Recurrent Neural Networks}


\section{Proofs}
\label{sec:proofs}

To show theorem \ref{thm:main-main}, we first consider the most general case in which $d_r$ is defined (Theorem \ref{thm:main}). Then we discuss the mild assumptions under which we can reduce to the original limit (Proposition \ref{prop:assump}). Additionally, we introduce some notations that will be used throughout the proof. If
$v = (t, p) \in \mathcal{G}_{\tmop{un}}$ is a node in the unfolded graph, it has a corresponding node in the folded graph, which is denoted by $\bar{v} =
(\bar{t}, p)$.

\begin{thm}
\label{thm:main}
  Given an RNN cyclic graph and its unfolded representation $(\mathcal{G}_c,
  \mathcal{G}_{\tmop{un}})$, we denote $C (\mathcal{G}_c)$ the set of directed
  cycles in $\mathcal{G}_c$. For $\vartheta \in C (\mathcal{G}_c)$, denote $l
  (\vartheta)$ the length of $\vartheta$ and $\sigma_s (\vartheta)$ the sum of
  $\sigma$ along $\vartheta$. Write $d_i = \limsup_{k \rightarrow \infty}
  \frac{\mathfrak{D}_i (n)}{n}$.\footnote{$\mathfrak{D}_i(n)$ is not defined when there does not exist a path from time $i$ to time $i+n$. We simply omit undefined cases when we consider the limsup. In a more rigorous sense, it is the limsup of a subsequence of $\{\mathfrak{D}_i(n)\}_{n=1}^{\infty}$, where $\mathfrak{D}_i(n)$ is defined.} we have :
  \begin{itemize}
    \item  The quantity $d_i$ is periodic, in the sense that $d_{i + m} = d_i,
    \forall i \in \mathbb{N}$.
    
    \item Let $d_r = \max_i d_i$, then
    \begin{equation}
    \label{eqn:recdepth2}
        d_r = \max_{\vartheta \in C (\mathcal{G}_c)} \frac{l
       (\vartheta)}{\sigma_s (\vartheta)}
    \end{equation}
  \end{itemize}
\end{thm}

\begin{proof}
  The first statement is easy to prove. Because of the periodicity of the graph,
  any path from time step \ $i$ to $i + n_{}$ corresponds to an isomorphic
  path from time step $i + m$ to $i + m + n$. Passing to limit, and we can
  deduce the first statement.
  
   Now we prove the second statement. Write $\vartheta_0 =
  \tmop{argmax}_{\vartheta} \frac{l (\vartheta)}{\sigma_s (\vartheta)} $.
  First we prove that $d \geq \frac{l (\vartheta_0)}{\sigma_s (\vartheta_0)}$.
  Let $c_1 = (t_1, p_1) \in \mathcal{G}_{\tmop{un}}$ be a node such that if we
  denote $\overline{c_1} = (\overline{t_1}, p_1)$ the image of $c_1$ on the
  cyclic graph, we have $\overline{c_1} \in \vartheta_0$. Consider the
  subsequence $S_0 = \left\{ \frac{\mathfrak{D}_{\overline{t_1}} (k \sigma_s
  (\vartheta_0))}{k \sigma_s (\vartheta_0)} \right\}_{k = 1}^{\infty}$ of
  $\left\{ \frac{\mathfrak{D}_{\overline{t_1}} (n)}{n} \right\}_{n =
  1}^{\infty}$. From the definition of $\mathfrak{D}$ and the fact that
  $\vartheta_0$ is a directed circle, we have $\mathfrak{D}_{\overline{t_1}}
  (k \sigma_s (\vartheta_0)) \geq k l (\vartheta_0)$, by considering the path
  on $\mathcal{G}_{\tmop{un}}$ corresponding to following $\vartheta_0$ $k$
  -times. So we have
  \[ d_r \geq \limsup_{k \rightarrow + \infty} \frac{\mathfrak{D}_i (n)}{n}
     \geq \limsup_{k \rightarrow + \infty} \frac{\mathfrak{D}_{\overline{t_1}} (k
     \sigma_s (\vartheta_0))}{k \sigma_s (\vartheta_0)} \geq \frac{k l
     (\vartheta_0)}{k \sigma_s (\vartheta_0)} = \frac{l
     (\vartheta_0)}{\sigma_s (\vartheta_0)} \]
  Next we prove $d_r \leq \frac{l (\vartheta_0)}{\sigma_s (\vartheta_0)}$. It
  suffices to prove that, for any $\epsilon \geq 0$, there exists $N > 0$,
  such that for any path $\gamma : \{ \nobracket (t_0, p_0) \nocomma, (t_1,
  p_1), \cdots, (t_{n_{\gamma}}, p_{n_{\gamma}}) \} \nobracket$ with $t_{n_\gamma} -
  t_1 > N$, we have $\frac{n_{\gamma}}{t_{n_\gamma} - t_1} \leq \frac{l
  (\vartheta_0)}{\sigma_s (\vartheta_0)} + \epsilon$. We denote $\bar{\gamma}$
  as the image of $\gamma$ on the cyclic graph. $\bar{\gamma}$ is a walk with
  repeated nodes and edges. Also, we assume there are in total $\Gamma$ nodes
  in cyclic graph $\mathcal{G}_c$.
  
  We first decompose $\bar{\gamma}$ into a path and a set of directed
  cycles. More precisely, there is a path $\gamma_0$ and a sequence of
  directed cycles $C = C_1 (\gamma), C_2 (\gamma), \cdots, C_w (\gamma)$ on
  $\mathcal{G}_c$ such that:
  \begin{itemize}
    \item The starting and end nodes of $\gamma_0$ is the same as $\gamma$.
    (If $\gamma$ starts and ends at the same node, take $\gamma_0$ as empty.)
    
    \item The catenation of the sequences of directed edges $E (\gamma_0), E
    (C_1 (\gamma)), E (C_2 (\gamma)), \cdots, E (C_w (\gamma))$ is a
    permutation of the sequence of edges of $E (\gamma)$.
  \end{itemize}
  The existence of such a decomposition can be proved iteratively by removing
  directed cycles from $\gamma$. Namely, if $\gamma$ is not a paths, there
  must be some directed cycles $C'_{}$ on $\gamma$. Removing $C'$ from
  $\gamma$, we can get a new walk $\gamma'$. Inductively apply this removal,
  we will finally get a (possibly empty) path and a sequence of directed
  cycles. For a directed path or loop $\gamma$, we write $D (\gamma)$ the
  distance between the ending node and starting node when travel through
  $\gamma$ once. We have
  \[ D (\gamma_0) : = \overline{t_{n_{\gamma}}} - \overline{t_0} + \sum_{i =
     1}^{| \gamma_0 |} \sigma (e_i) \]
  where $e_i, i \in \{ 1, 2, \cdots, | \gamma_0 | \}$ is all the edges of
  $\gamma_0$. $\bar{t}$ denotes the module of $t$: $t \equiv \bar{t}
  (\tmop{mod} m)$.
  
  So we have:
  \[ | D (\gamma_0) | \leq m + \Gamma \cdot \max_{e \in \mathcal{G}_c} \sigma
     (e) = M \]
  \ For convenience, we denote $l_0, l_1, \cdots, l_w$ to be the length of
  path $\gamma_0$ and directed cycles $C_1 (\gamma), C_2 (\gamma), \cdots, C_w
  (\gamma)$. Obviously we have:
  \[ n_{\gamma} = \sum_{i = 0}^w l_i \]
  And also, we have
  \[ t_{n_\gamma} - t_1 = \sum_{i = 1}^w \sigma_s (C_i) + D (\gamma_0) \]
  So we have:
  \[ \frac{n_{\gamma}}{t_{n_\gamma} - t_1} = \frac{l_0}{t_{n_\gamma} - t_1} + \sum_{i = 1}^w
     \frac{l_i}{t_{n_\gamma} - t_1} \leq \frac{\Gamma}{N} + \sum_{i = 1}^w
     \frac{l_i}{t_{n_\gamma} - t_1} \]
  In which we have for all $i \in \{ 1, 2, \cdots, w \}$ :
  \[ \frac{l_i}{t_{n_\gamma} - t_1} = \frac{l_i}{\sigma_s (C_i)} \cdot \frac{\sigma_s
     (C_i)}{t_{n_\gamma} - t_1} \leq \frac{l (\vartheta_0)}{\sigma_s (\vartheta_0)}
     \frac{\sigma_s (C_i)}{t_{n_\gamma} - t_1} \]
  So we have:
  \[ \sum_{i = 1}^w \frac{l_i}{t_{n_\gamma} - t_1} \leq \frac{l
     (\vartheta_0)}{\sigma_s (\vartheta_0)} \left[ 1 - \frac{D (\gamma_0)}{t_{n_\gamma}
     - t_1} \right] \leq \frac{l (\vartheta_0)}{\sigma_s (\vartheta_0)} +
     \frac{M'}{N} \]
  in which $M'$ and $\Gamma$ are constants depending only on the RNN
  $\mathcal{G}_c$.
  
  Finally we have:
  \[ \frac{n_{\gamma}}{t_{n_\gamma} - t_1} \leq \frac{l (\vartheta_0)}{\sigma_s
     (\vartheta_0)} + \frac{M' + \Gamma}{N} \]
  take $N > \frac{M' + \Gamma}{\epsilon}$, we can prove the fact that $d_r
  \leq \frac{l (\vartheta_0)}{\sigma_s (\vartheta_0)}$.
  
  \ 
\end{proof}

\begin{proposition}
\label{prop:assump}
  Given an RNN and its two graph representations $\mathcal{G}_{\tmop{un}}$ and
  $\mathcal{G}_c$, if $\exists \vartheta \in C (\mathcal{G}_c)$ such that
  $(1)$ $\vartheta$ achieves the maximum in Eq.(\ref{eqn:recdepth2}) and $(2)$
  the corresponding path of $\vartheta$ in $\mathcal{G}_{\tmop{un}}$ visits nodes at every time step,
  then we have
  \[ d_r = \max_{i \in \mathbb{Z}} \left( \limsup_{n \rightarrow + \infty}
     \frac{\mathfrak{D}_i (n)}{n} \right) = \lim_{n \rightarrow + \infty}
     \frac{\mathfrak{D}_i (n)}{n} \]
\end{proposition}

\begin{proof}
  We only need to prove, in such a graph, for all $i \in \mathbb{Z}$ we have
  \[ \liminf_{n \rightarrow + \infty} \frac{\mathfrak{D}_i (n)}{n} \geq
     \max_{i \in \mathbb{Z}} \left( \limsup_{n \rightarrow + \infty}
     \frac{\mathfrak{D}_i (n)}{n} \right) = d_r \]
  Because it is obvious that
  \[ \tmop{liminf}_{n \rightarrow + \infty} \frac{\mathfrak{D}_i (n)}{n} \leq
     d_r \]
  Namely, it suffice to prove, for all $i \in \mathbb{Z}$, for all $\epsilon
  > 0$, there is an $N_{\epsilon} > 0$, such that when $n > N_{\epsilon}$, we
  have $\frac{\mathfrak{D}_i (n)}{n} \geq d_r - \epsilon$. On the other hand,
  for $k \in \mathbb{N}$, if we assume $(k + 1) \sigma_s (\vartheta) + i > n
  \geq i + k \cdot \sigma_s (\vartheta)$, then according to condition $(2)$ we
  have
  \[ \frac{\mathfrak{D}_i (n)}{n} \geq \frac{k \cdot l (\vartheta)}{(k + 1)
     \sigma_s (\vartheta)} = \frac{l (\vartheta)}{\sigma_s (\vartheta)} -
     \frac{l (\vartheta)}{\sigma_s (\vartheta)} \frac{1}{k + 1} \]
  We can see that if we set $k > \frac{\sigma_s (\vartheta)}{l (\vartheta)
  \epsilon}$, the inequality we wanted to prove.
  
  \ 
\end{proof}

We now prove Proposition \ref{prop:sup} and Theorem \ref{thm:feed} as follows.


\begin{proposition}
  Given an RNN with recurrent depth $d_r$, we denote
  \[ d_f = \sup_{i, n \in \mathbb{Z}} \mathfrak{D}_i^{\ast} (n) - n \cdot
     d_r. \]
  The supremum $d_f$ exists and we have the following least upper bound:
  \[ \mathfrak{D}_i^{\ast} (n) \leq n \cdot d_r + d_f. \]
\end{proposition}

\begin{proof}
  We first prove that $d_f < + \infty$. Write $d_f (i) = \sup_{n \in
  \mathbb{Z}} \mathfrak{D}_i^{\ast} (n) - n \cdot d_r$. It is easy to verify
  $d_f (\cdot)$ is $m -$periodic, so it suffices to prove for each $i \in
  \mathbb{N}$, $d_f (i) < + \infty$. Hence it suffices to prove
  \[ \limsup_{n \rightarrow \infty} (\mathfrak{D}_i^{\ast} (n) - n \cdot d_r)
     < + \infty. \]
  From the definition, we have
  $\mathfrak{D}_i (n) \geq \mathfrak{D}_i^{\ast} (n).$
  So we have
  \[ \mathfrak{D}_i^{\ast} (n) - n \cdot d_r \leq \mathfrak{D}_i (n) - n
     \cdot d_r. \]
  From the proof of Theorem \ref{thm:main}, \ there exists two constants $M'$ and
  $\Gamma$ depending only on the RNN $\mathcal{G}_c$, such that
  \[ \frac{\mathfrak{D}_i (n)}{n} \leq d_r + \frac{M' + \Gamma}{n}. \]
  So we have
  \[ \limsup_{n \rightarrow \infty} (\mathfrak{D}_i^{\ast} (n) - n \cdot d_r)
     \leq \limsup_{n \rightarrow \infty} (\mathfrak{D}_i (n) - n \cdot d_r)
     \leq M' + \Gamma. \]
  Also, we have $d_f = \sup_{i, n \in \mathbb{Z}} \mathfrak{D}_i^{\ast} (n) -
  n \cdot d_r$, so for any $i, n \in \mathbb{Z}$,
  \[ d_f \geq \mathfrak{D}_i^{\ast} (n) - n \cdot d_r. \]
  
\end{proof}

\begin{thm}
  Given an RNN and its two graph representations $\mathcal{G}_{\tmop{un}}$ and
  $\mathcal{G}_c$, we denote $\xi (\mathcal{G}_c)$ the set of directed path
  that starts at an input node and ends at an output node in $\mathcal{G}_c$.
  For $\gamma \in \xi(\mathcal{G}_c)$, denote $l (\gamma)$ the length and
  $\sigma_s (\gamma)$ the sum of $\sigma$ along $\gamma$. Then we have:
  \[ d_f = \sup_{i, n \in \mathbb{Z}} \mathfrak{D}_i^{\ast} (n) - n \cdot d_r
     = \max_{\gamma \in \xi (\mathcal{G}_c)} l (\gamma) - \sigma_s (\gamma)
     \cdot d_r. \]
\end{thm}

\begin{proof}
Let $\gamma : \{ \nobracket (t_0, 0) \nocomma, (t_1,
  p_1), \cdots, (t_{n_\gamma}, p) \} \nobracket$ be a path in $\mathcal{G}_{\tmop{un}}$ from an input node $(t_0, 0)$ to an output node $(t_{n_{\gamma}}, p)$, where $t_0 = i$ and $t_{n_\gamma} = i+n$. We denote $\bar{\gamma}$
  as the image of $\gamma$ on the cyclic graph. 
From the proof of Theorem \ref{thm:main}, for each $\bar{\gamma}$ in $\mathcal{G}_{c}$, we can decompose it into a path $\gamma_0$ and a sequence of directed cycles $C = C_1 (\gamma), C_2 (\gamma), \cdots, C_w (\gamma)$ on
  $\mathcal{G}_c$ satisfying those properties listed in Theorem \ref{thm:main}.
We denote $l_0, l_1, \cdots, l_w$ to be the length of
  path $\gamma_0$ and directed cycles $C_1 (\gamma), C_2 (\gamma), \cdots, C_w
  (\gamma)$. We know $\frac{l_k}{\sigma_s(C_k)} \leq d_r$ for all $k = 1,2,\dots,w$ by definition. Thus,
\begin{align*}
    l_k \leq & \:d_r\cdot \sigma_s(C_k) \\
    \sum_{k=1}^w l_k \leq & \:d_r\cdot \sum_{k=1}^w  \sigma_s(C_k) 
\end{align*}
Note that $n = \sigma_s(\gamma_0) + \sum_{k=1}^w  \sigma_s(C_k) $. Therefore,
\begin{align*}
    l(\gamma) - n\cdot d_r = &\:l_0 +\sum_{k=1}^w l_k- n\cdot d_r \\\leq & \:l_0+d_r\cdot (\sum_{k=1}^w  \sigma_s(C_k)-n)
    \\= & \: l_0- d_r \cdot \sigma_s(\gamma_0)
\end{align*}
for all time step $i$ and all integer $n$. The above inequality suggests that in order to take the supremum over all paths in $\mathcal{G}_{\tmop{un}}$, it suffices to take the maximum over a directed path in $\mathcal{G}_c$. On the other hand, the equality can be achieved simply by choosing the corresponding path of $\gamma_0$ in $\mathcal{G}_{\tmop{un}}$. The desired conclusion then follows immediately.

\end{proof}

Lastly, we show Theorem \ref{thm:rsc}.

\begin{thm}
\label{thm:main2}
  Given an RNN cyclic graph and its unfolded representation $(\mathcal{G}_c,
  \mathcal{G}_{\tmop{un}})$, we denote $C (\mathcal{G}_c)$ the set of directed
  cycles in $\mathcal{G}_c$. For $\vartheta \in C (\mathcal{G}_c)$, denote $l
  (\vartheta)$ the length of $\vartheta$ and $\sigma_s (\vartheta)$ the sum of
  $\sigma$ along $\vartheta$. Write $s_i = \lim \inf_{k \rightarrow \infty}
  \frac{\mathfrak{d}_i (n)}{n}$. We have :
  \begin{itemize}
    \item  The quantity $s_i$ is periodic, in the sense that $s_{i + m} = s_i,
    \forall i \in \mathbb{N}$.
    
    \item Let $s = \min_i s_i$, then
    \begin{equation}
    \label{eqn:main2}
        d_r = \min_{\vartheta \in C (\mathcal{G}_c)} \frac{l
       (\vartheta)}{\sigma_s (\vartheta)}.
    \end{equation}
  \end{itemize}
\end{thm}
\begin{proof}
  The proof is essentially the same as the proof of the first theorem. So we
  omit it here. 
\end{proof}

\begin{proposition}
\label{prop:assump2}
  Given an RNN and its two graph representations $\mathcal{G}_{\tmop{un}}$ and
  $\mathcal{G}_c$, if $\exists \vartheta \in C (\mathcal{G}_c)$ such that
  $(1)$ $\vartheta$ achieves the minimum in Eq.(\ref{eqn:main2}) and $(2)$ the
  corresponding path of $\vartheta$ in $\mathcal{G}_{\tmop{un}}$ visits nodes at every time step,
  then we have
  \[ s = \min_{i \in \mathbb{Z}} \left( \liminf_{n \rightarrow + \infty}
     \frac{\mathfrak{d}_i (n)}{n} \right) = \lim_{n \rightarrow + \infty}
     \frac{\mathfrak{d}_i (n)}{n}. \]
\end{proposition}
\begin{proof}
  The proof is essentially the same as the proof of the Proposition \ref{prop:assump}. So we
  omit it here. 
\end{proof}

\newpage



\newpage
\section{Experiment Details}
\subsection{RNNs with $\tanh$}
In this section we explain the functional dependency among nodes in RNNs with $\tanh$ in detail.

The transition function for each node is the $\tanh$ function. The output of a node $v$ is a vector $h_v$. To compute the output for a node, we simply take all incoming nodes as input, and sum over their affine transformations and then apply the $\tanh$ function (we omit the bias term for simplicity).
\begin{equation*}
    h_v = \mathrm{tanh}\left(\sum_{u \in \mathrm{In}(v)}\textbf{W}(u)h_u\right),
\end{equation*}
where $\textbf{W}(\cdot)$ represents a real matrix.

\begin{figure}[htp]
\center
\includegraphics[width=5cm]{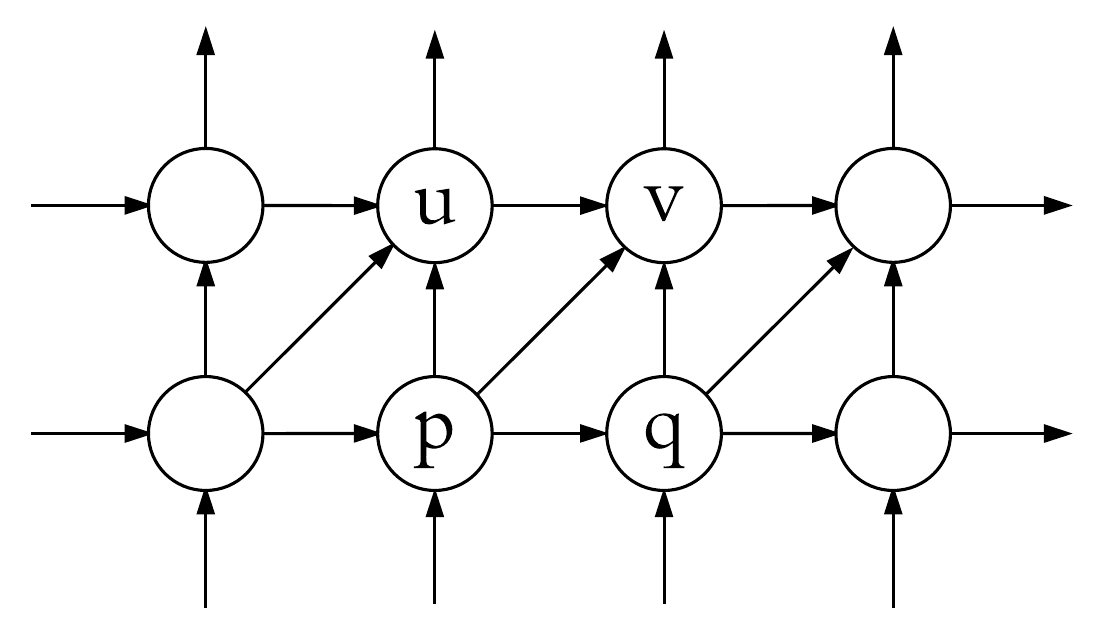}
\vspace{-10pt}
\caption{``Bottom-up'' architecture ($bu$).}
\label{fig:bu_ex}
\end{figure}
As a more concrete example, consider the ``bottom-up'' architecture in Figure \ref{fig:bu_ex}, with which we did the experiment described in Section \ref{sec:depth_nontrivial}. To compute the output of node $v$, 
\begin{equation}
h_v = \mathrm{tanh}(\textbf{W}(u)h_u+\textbf{W}(p)h_p+\textbf{W}(q)h_q).
\end{equation}

\subsection{LSTMs}
\label{sec:LSTM}
In this section we explain the Multidimensional LSTM (introduced by \cite{Graves2007}) which we use for experiments with LSTMs.

The output of a node $v$ of the LSTM is a 2-tuple ($c_v$,$h_v$), consisting of a cell memory state $c_v$ and a hidden state $h_v$. The transition function $F$ is applied to each node indistinguishably. We describe the computation of $F$ below in a sequential manner (we omit the bias term for simplicity). 
%\[\arraycolsep=2.4pt\def\arraystretch{2.2}
\begin{align*}
z &= g\left(\sum_{u \in \mathrm{In}(v)}\textbf{W}_z(u)h_u\right) \qquad &\text{block input} \\
i &= \sigma\left(\sum_{u \in \mathrm{In}(v)}\textbf{W}_i(u)h_u\right) \qquad &\text{input gate} \\
o &= \sigma\left(\sum_{u \in \mathrm{In}(v)}\textbf{W}_o(u)h_u\right) \qquad &\text{output gate} \\
\{f_u\} &= \left\{\sigma\left(\sum_{u' \in \mathrm{In}(v)}\textbf{W}_{f_u}(u')h_u\right)|u \in \mathrm{In}(v)\right\} \qquad &\text{A set of forget gates}\\
c_v &= i \odot z + \sum_{u \in \mathrm{In}(v)} f_u \odot c_u  \qquad &\text{cell state} \\
h_v &= o \odot c_v&  \qquad  \text{hidden state}
\end{align*}

Note that the Multidimensional LSTM includes the usual definition of LSTM as a special case, where the extra forget gates are 0 (i.e., bias term set to -$\infty$) and extra weight matrices are 0. We again consider the architecture $bu$ in Fig. \ref{fig:bu_ex}. We first compute the block input, the input gate and the output gate by summing over all affine transformed outputs of $u,p,q$, and then apply the activation function. For example, to compute the input gate, we have
\begin{equation*}
    i = \sigma\left(\textbf{W}_i(u)h_u+\textbf{W}_i(p)h_p+\textbf{W}_i(q)h_q\right).
\end{equation*}
Next, we compute one forget gate for each pair of $(v,u), (v,p), (v,q)$. The way of computing a forget gate is the same as computing the other gates. For example, the forget gate in charge of the connection of $u \to v$ is computed as,
\begin{equation*}
    f_u= \sigma\left(\textbf{W}_{f_u}(u)h_u+\textbf{W}_{f_u}(p)h_u+\textbf{W}_{f_u}(q)h_u\right).
\end{equation*}
Then, the cell state is simply the sum of all element-wise products of the input gate with the block output and forget gates with the incoming nodes' cell memory states,
\begin{equation*}
    c_v = i \odot z + f_u \odot c_u+f_p \odot c_p+f_q \odot c_q.
\end{equation*}
Lastly, the hidden state is computed as usual,
\begin{equation*}
h_v = o \odot c_v.
\end{equation*}


%\label{sec:exp_details}
%In this section, we show experimental details
%including all the learning curves and the function dependencies of architectures in each experiment
%(the general function dependencies of LSTMs have been shown in Section \ref{sec:LSTM}; here,
% we focus on $\tanh$).

\subsection{Recurrent Depth is Non-trivial}
\label{sec:exp_dr_nontrivial}
The validation curves of the 4 different connecting
architectures $sh$, $st$, $bu$ and $td$ on text8
dataset for both $\tanh$RNN-small and LSTM-small are shown below:
\begin{figure}[htp]
\center
\includegraphics[width=350pt]{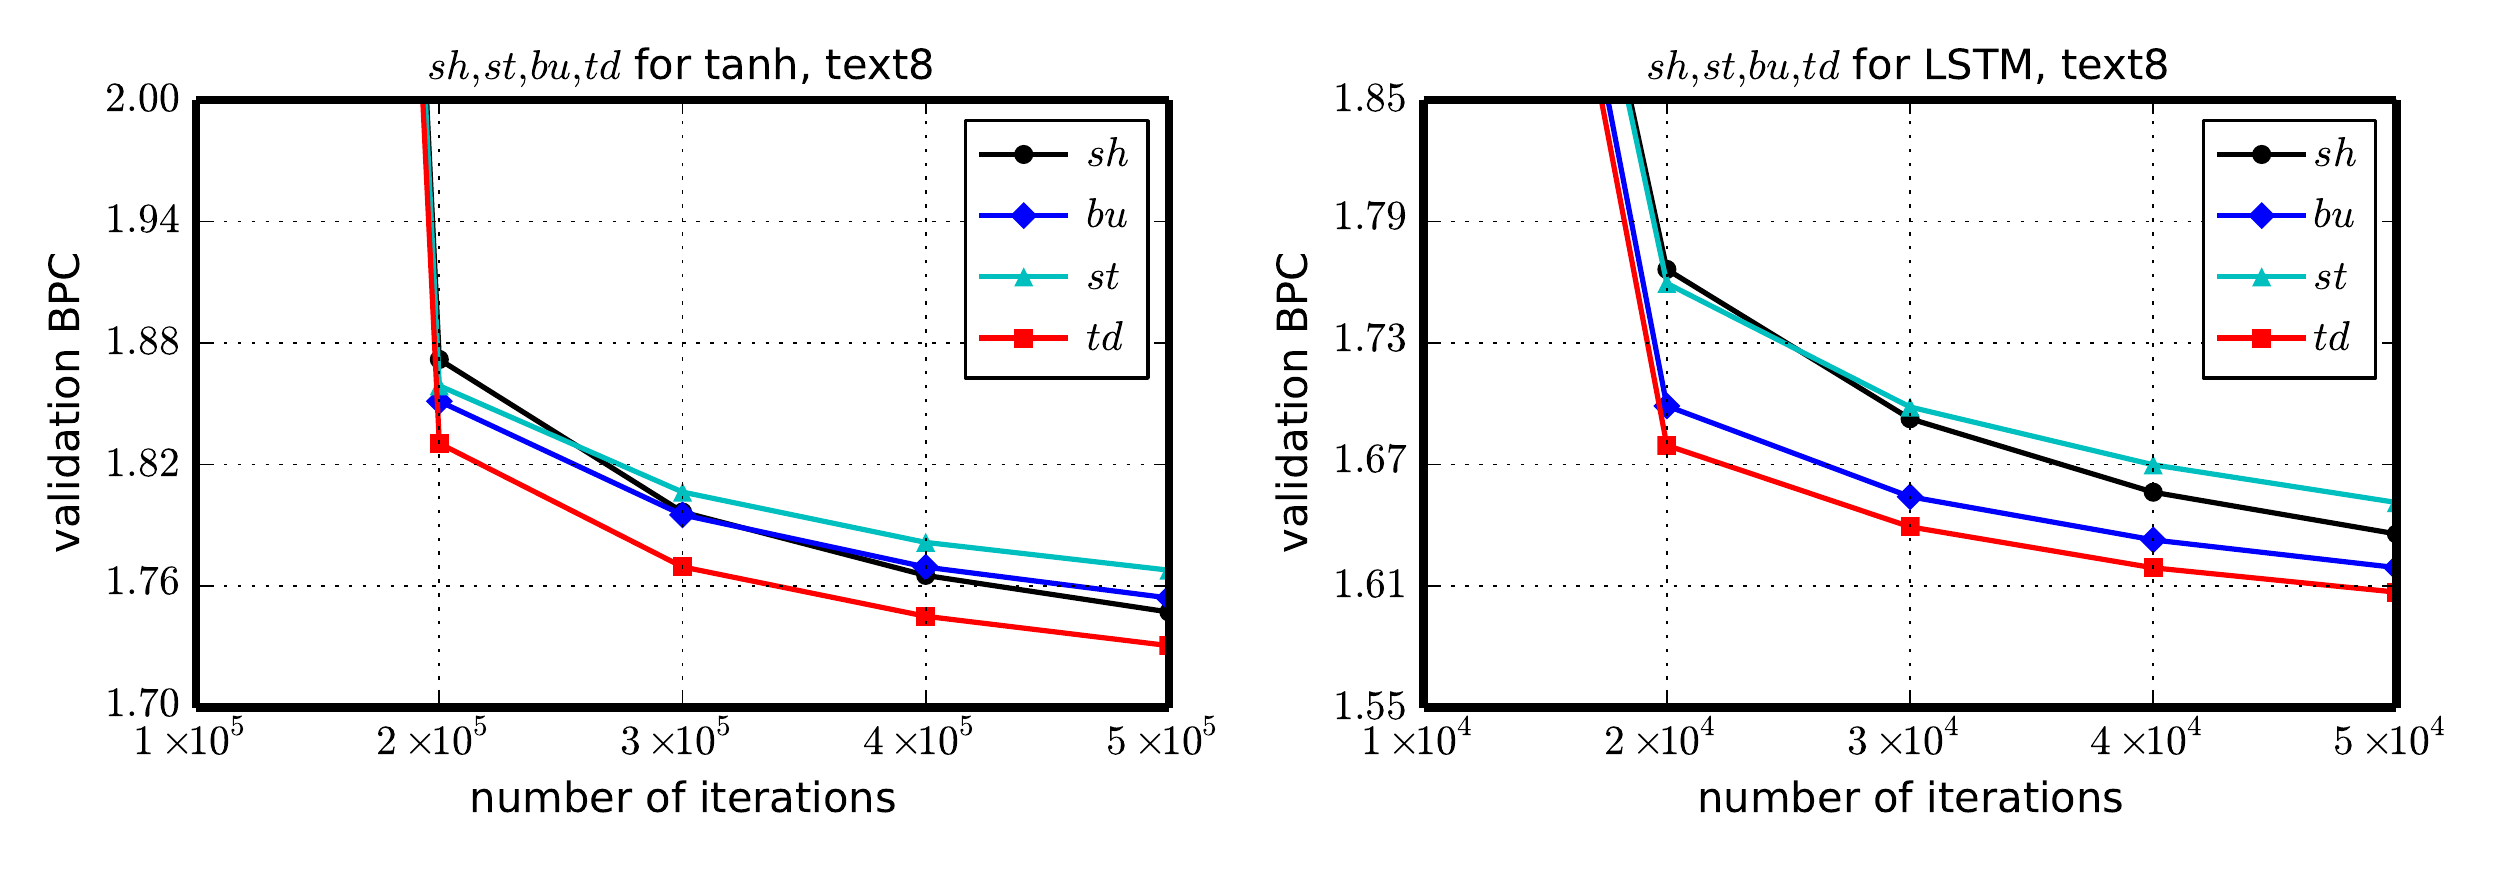}
\vspace{-10pt}
\caption{Validation curves for $sh$, $st$, $bu$ and $td$ on test8 dataset.
Left: results for $\tanh$RNN-small. Right: results for LSTM-small.}
\label{fig:butd_ex}
\end{figure}

\subsection{Full Comparisons on Depths}
\label{sec:full_com}
Figure \ref{fig:3x3lm_ex}
shows all the validation curves for the 9 architectures on text8 dataset, with
their $d_r = 1, 2, 3$ and $d_f = 2, 3, 4$ respectively.
We initialize hidden-to-hidden
matrices from uniform distribution.
%we observe that orthogonal intialization helps for the optimization
%issues when $d_f$ is large, in which increasing $d_f$ does not harm the learning. 
%While the results are still consistent with our analysis in the main paper.
%Notice that one can achieve better results with much larger models
%on this dataset, as in \cite{mikolov2012subword}. 

\begin{figure}[htp]
\center
\includegraphics[width=\textwidth]{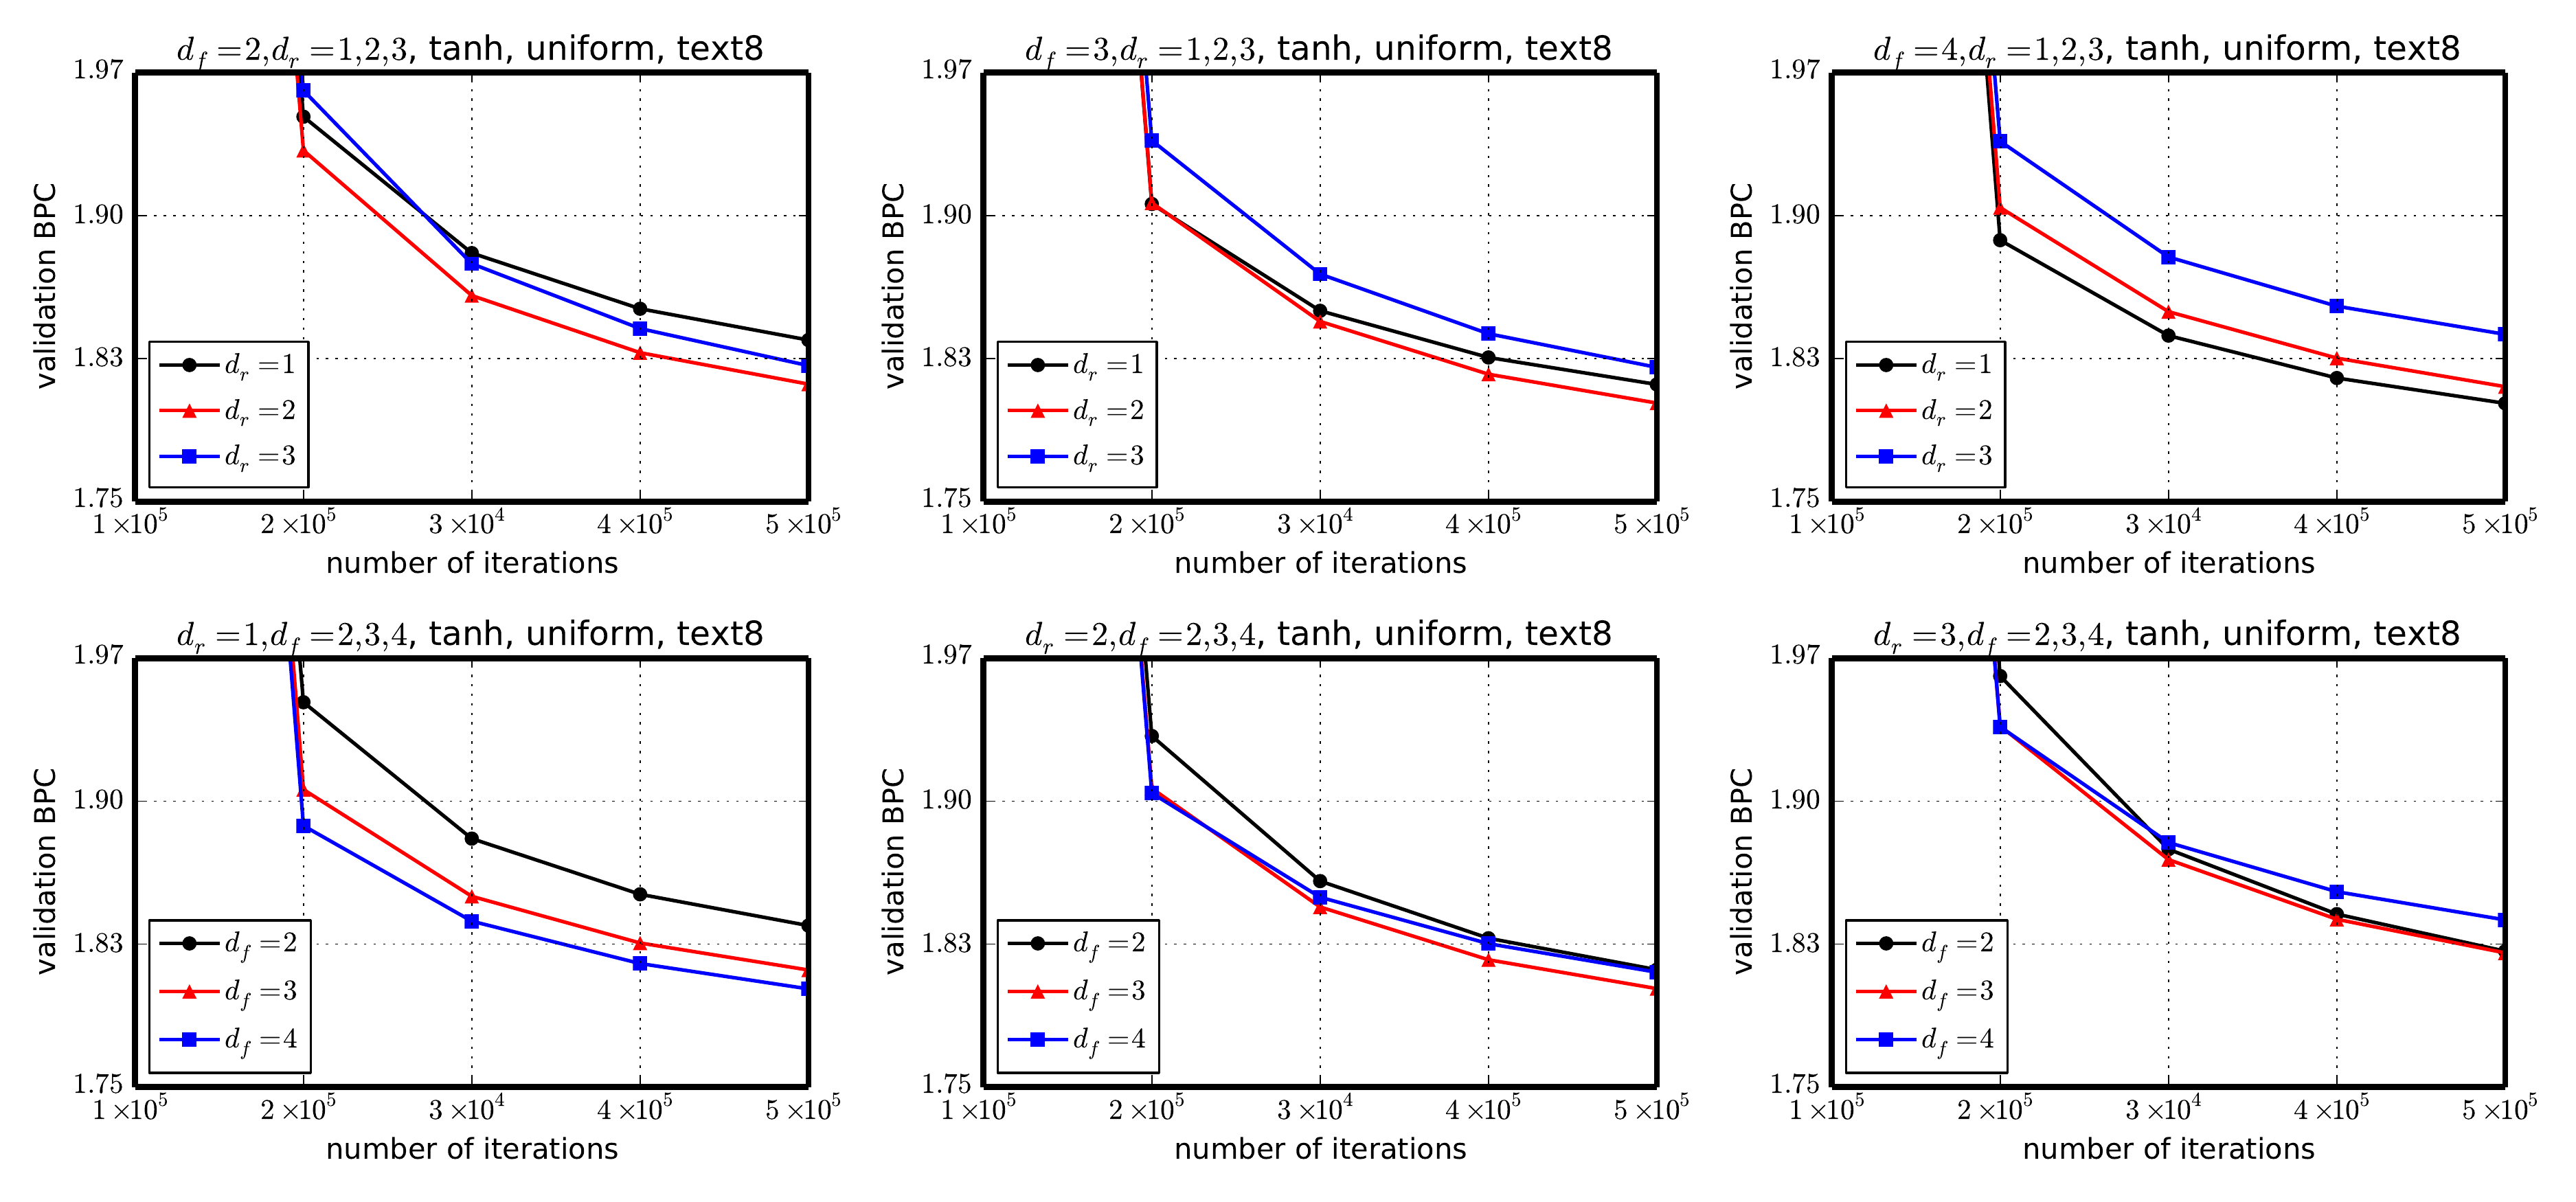}
\vspace{-10pt}
\caption{Validation curves of 9 architectures with feedforward depth $d_f = 2, 3, 4$
and recurrent depth $d_r = 1, 2, 3$ on test8 dataset.
For each figure in the first row, we fix $d_f$ and draw $3$ curves with different $d_r=1, 2, 3$.
For each figure in the second row, we fix $d_r$ and draw $3$ curves with different $d_f=2, 3, 4$.
}
\label{fig:3x3lm_ex}
\end{figure}

%\begin{figure}[htp]
%\center
%\includegraphics[width=\textwidth]{./figures/3x3_ml_ortho_appendix.pdf}
%\vspace{-10pt}
%\caption{Validation curves of 9 architectures with feedforward depth $d_f = 2, 3, 4$
%and recurrent depth $d_r = 1, 2, 3$ on test8 dataset.
%\textbf{Hidden-to-hidden matrices are initialized using orthogonal matrices.}
%For each figure in the first row, we fix $d_r$ and draw $3$ curves with different $d_f=2, 3, 4$.
%For each figure in the second row, we fix $d_f$ and draw $3$ curves with different $d_r=2, 3, 4$.
%}
%\label{fig:3x3ml_ortho_ex}
%\end{figure}
%In each figure in the first row, we fix feedforward depth $d_f$, and
%plot the curves for $d_r = 1, 2, 3$.
%In each figure in the second row, we fix feedforward depth $d_r$, and
%plot the curves for $d_f = 1, 2, 3$.
%
%\subsection{Feedforward Depth On Long Term Dependency}

Also, to see if increasing feedforward depth/ recurrent depth helps
for long term dependency problems, 
we evaluate these 9 architectures on sequential MNIST task, with roughly the
same number of parameters(~8K, where the first architecture with $d_r=1$ and $d_f=2$ has hidden size of 90.). 
Hidden-to-hidden matrices
are initialized from uniform distribution.
%\begin{table}[h]
%\vspace{-15pt}
%\caption{test accs of 9 architectures with different $d_r$, $d_f$ for tanh}
%\label{tb:mnist9}
%\begin{center}
%\begin{small}
%\begin{sc}
%\begin{tabular}{c|@{\hspace{4pt}}c@{\hspace{6pt}}c@{\hspace{6pt}}c}
%\hline
%\hline
%%\abovespace\belowspace
%test acc($\%$)&$d_r = 1$ & $d_r = 2$ & $d_r = 3$\\
%\hline
% $d_f = 2$ & $35.0$ & $21.1$ & $11.4$\\
% $d_f = 3$ & $35.0$ & $11.3$ & $11.4$\\
% $d_f = 4$ & $\mathbf{35.2}$ & $11.4$ & $11.3$\\
%\hline
%\end{tabular}
%\end{sc}
%\end{small}
%\end{center}
%\vspace{-15pt}
%\end{table}

%This experiment is performed on MNIST (non-permuted version),
%all the models have the same architectures as in
%Section \ref{sec:full_com}. We first show that, when the intializition
%uses uniform distribution, increasing feedforward depth (``stacking layers", in another word)
%does not bring any benefit even does harm to the test performance: 
\begin{figure}[h]
\center
\includegraphics[width=\textwidth]{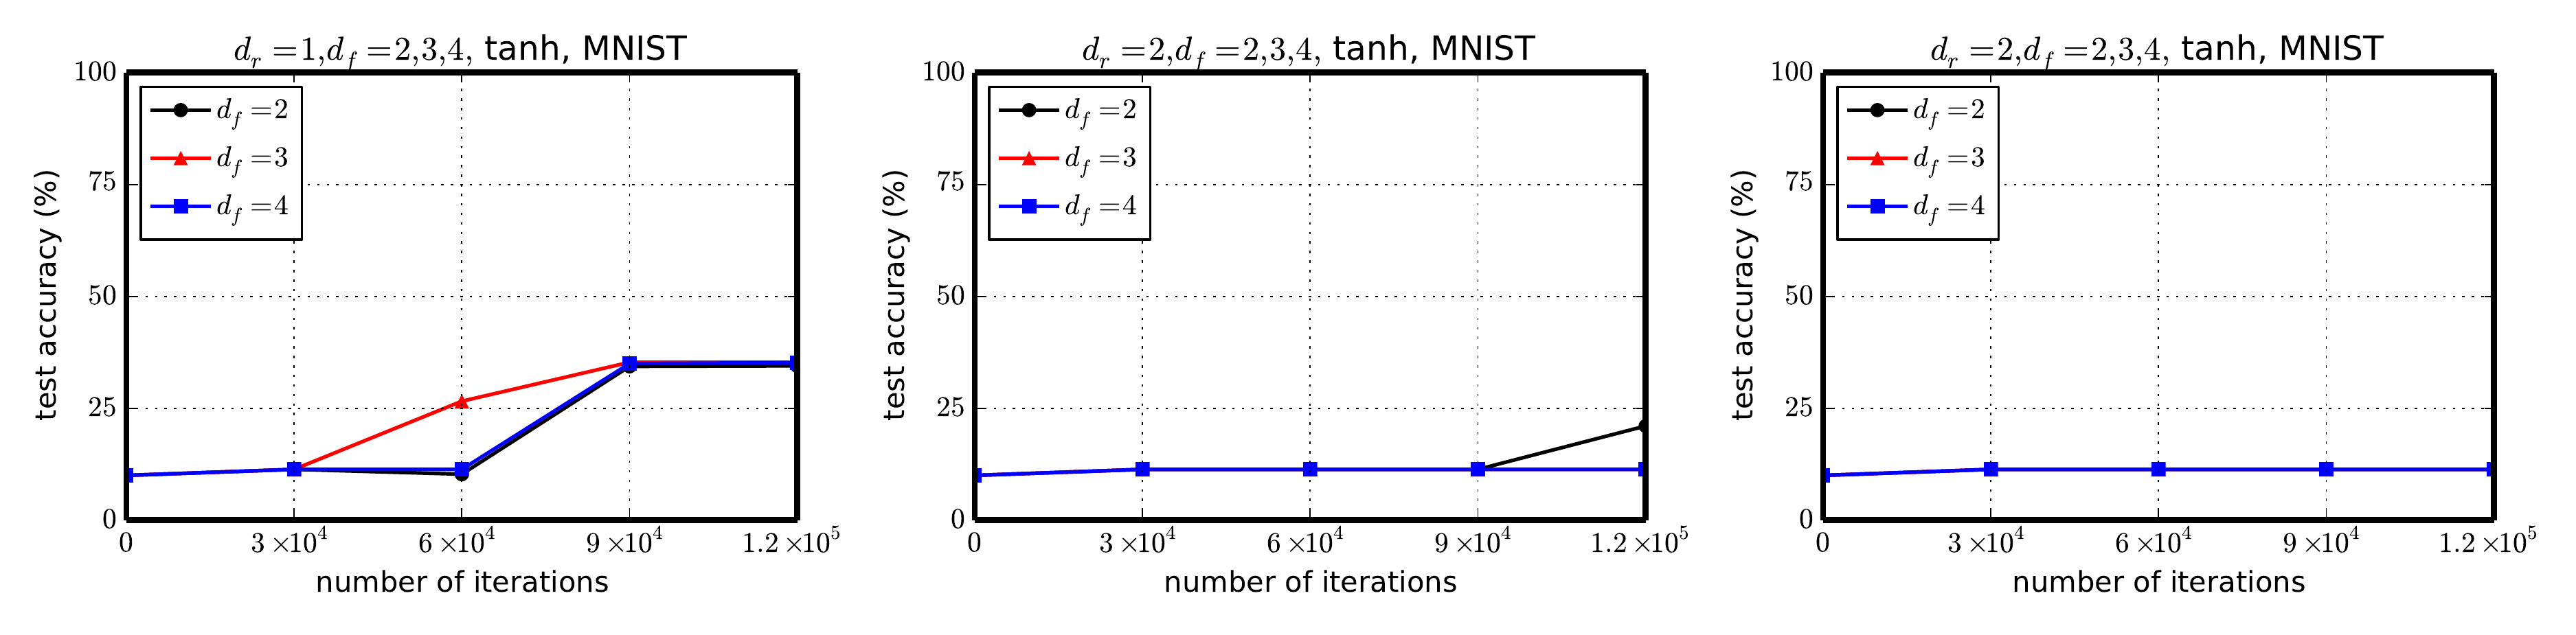}
\vspace{-10pt}
\caption{Test accuracies of 9 architectures with feedforward depth $d_f = 2, 3, 4$
and recurrent depth $d_r = 1, 2, 3$ on sequential MNIST. For each figure,
we fix $d_r$ and draw $3$ curves with different $d_f$.
}
\label{fig:3xxmnist_ex}
\end{figure}
%\begin{figure}[htp]
%\center
%\includegraphics[width=\textwidth]{./figures/3x3_mnist_ortho_appendix.pdf}
%\vspace{-10pt}
%\caption{Test accuracies of 9 architectures with feedforward depth $d_f = 2, 3, 4$
%and recurrent depth $d_r = 1, 2, 3$ on sequential MNIST. For each figure,
%we fix $d_r$ and draw $3$ curves with different $d_f$.
%\textbf{Hidden-to-hidden matrices are initialized using orthogonal matrices.}}
%\label{fig:3x3mnist_ortho_ex}
%\end{figure}


Figure \ref{fig:3xxmnist_ex}
clearly show that, 
as the feedforward depth
increases, the model performance stays roughly the same.
In addition, note that increasing recurrent depth might even result in performance decrease. 
This is possibly because that larger recurrent depth amplifies the gradient
vanishing/exploding problems, which is detrimental on long term
dependency tasks.
%YB: I did not understand the point:
%We argue that feedforward depth/recurrent depth might not necessarily be
%a proper measure of the model's behaviors in the long run,
%and above experiments provides evidences for our argument.

\newpage
\subsection{Recurrent Skip Coefficients}

The test curves for all the experiments are shown in Figure \ref{fig:mnist_ex}. 
In Figure \ref{fig:mnist_ex}, we observed that
obtaining good performance on MNIST requires larger $s$ than for pMNIST.
We hypothesize that this is because, for the sequential MNIST dataset, 
each training example contains many consecutive zero-valued subsequences, each of
length $10$ to $20$. Thus within those subsequences, the input-output gradient flow
could tend to vanish. However, when the recurrent skip coefficient is large enough to cover those
zero-valued subsequences, the model starts to perform better.
With $p$MNIST, even though the random permuted order seems harder to learn, the permutation on the other hand
blends zeros and ones to form more uniform sequences, and this may explain why training is easier, less hampered
by by the long sequences of zeros.

\subsection{Recurrent Skip Coefficients vs. Skip Connections}
Test curves for all the experiments are shown in Figure \ref{fig:verify_ex}.
Observe that in most cases,
the test accuracy of (3) is worse than (2) in the beginning
while beating (2) in the middle of the training.
This is possibly because in the first several time steps, it is easier
for (2) to pass information to the output thanks to the skip connections,
while only after multiples of $k$ time steps, (3) starts to show its
advantage with recurrent skip connections\footnote{It will be more clear if one checks the length
of the shortest path from an node at time $t$ to to a node at time $t+k$ in both architectures.}.
The shorter paths in (2) make its gradient flow more easily in the beginning,
but in the long run, (3) seems to be more superior, because of its more prominent skipping effect over time. 

\begin{figure}[htp]
\center
\includegraphics[width=350pt]{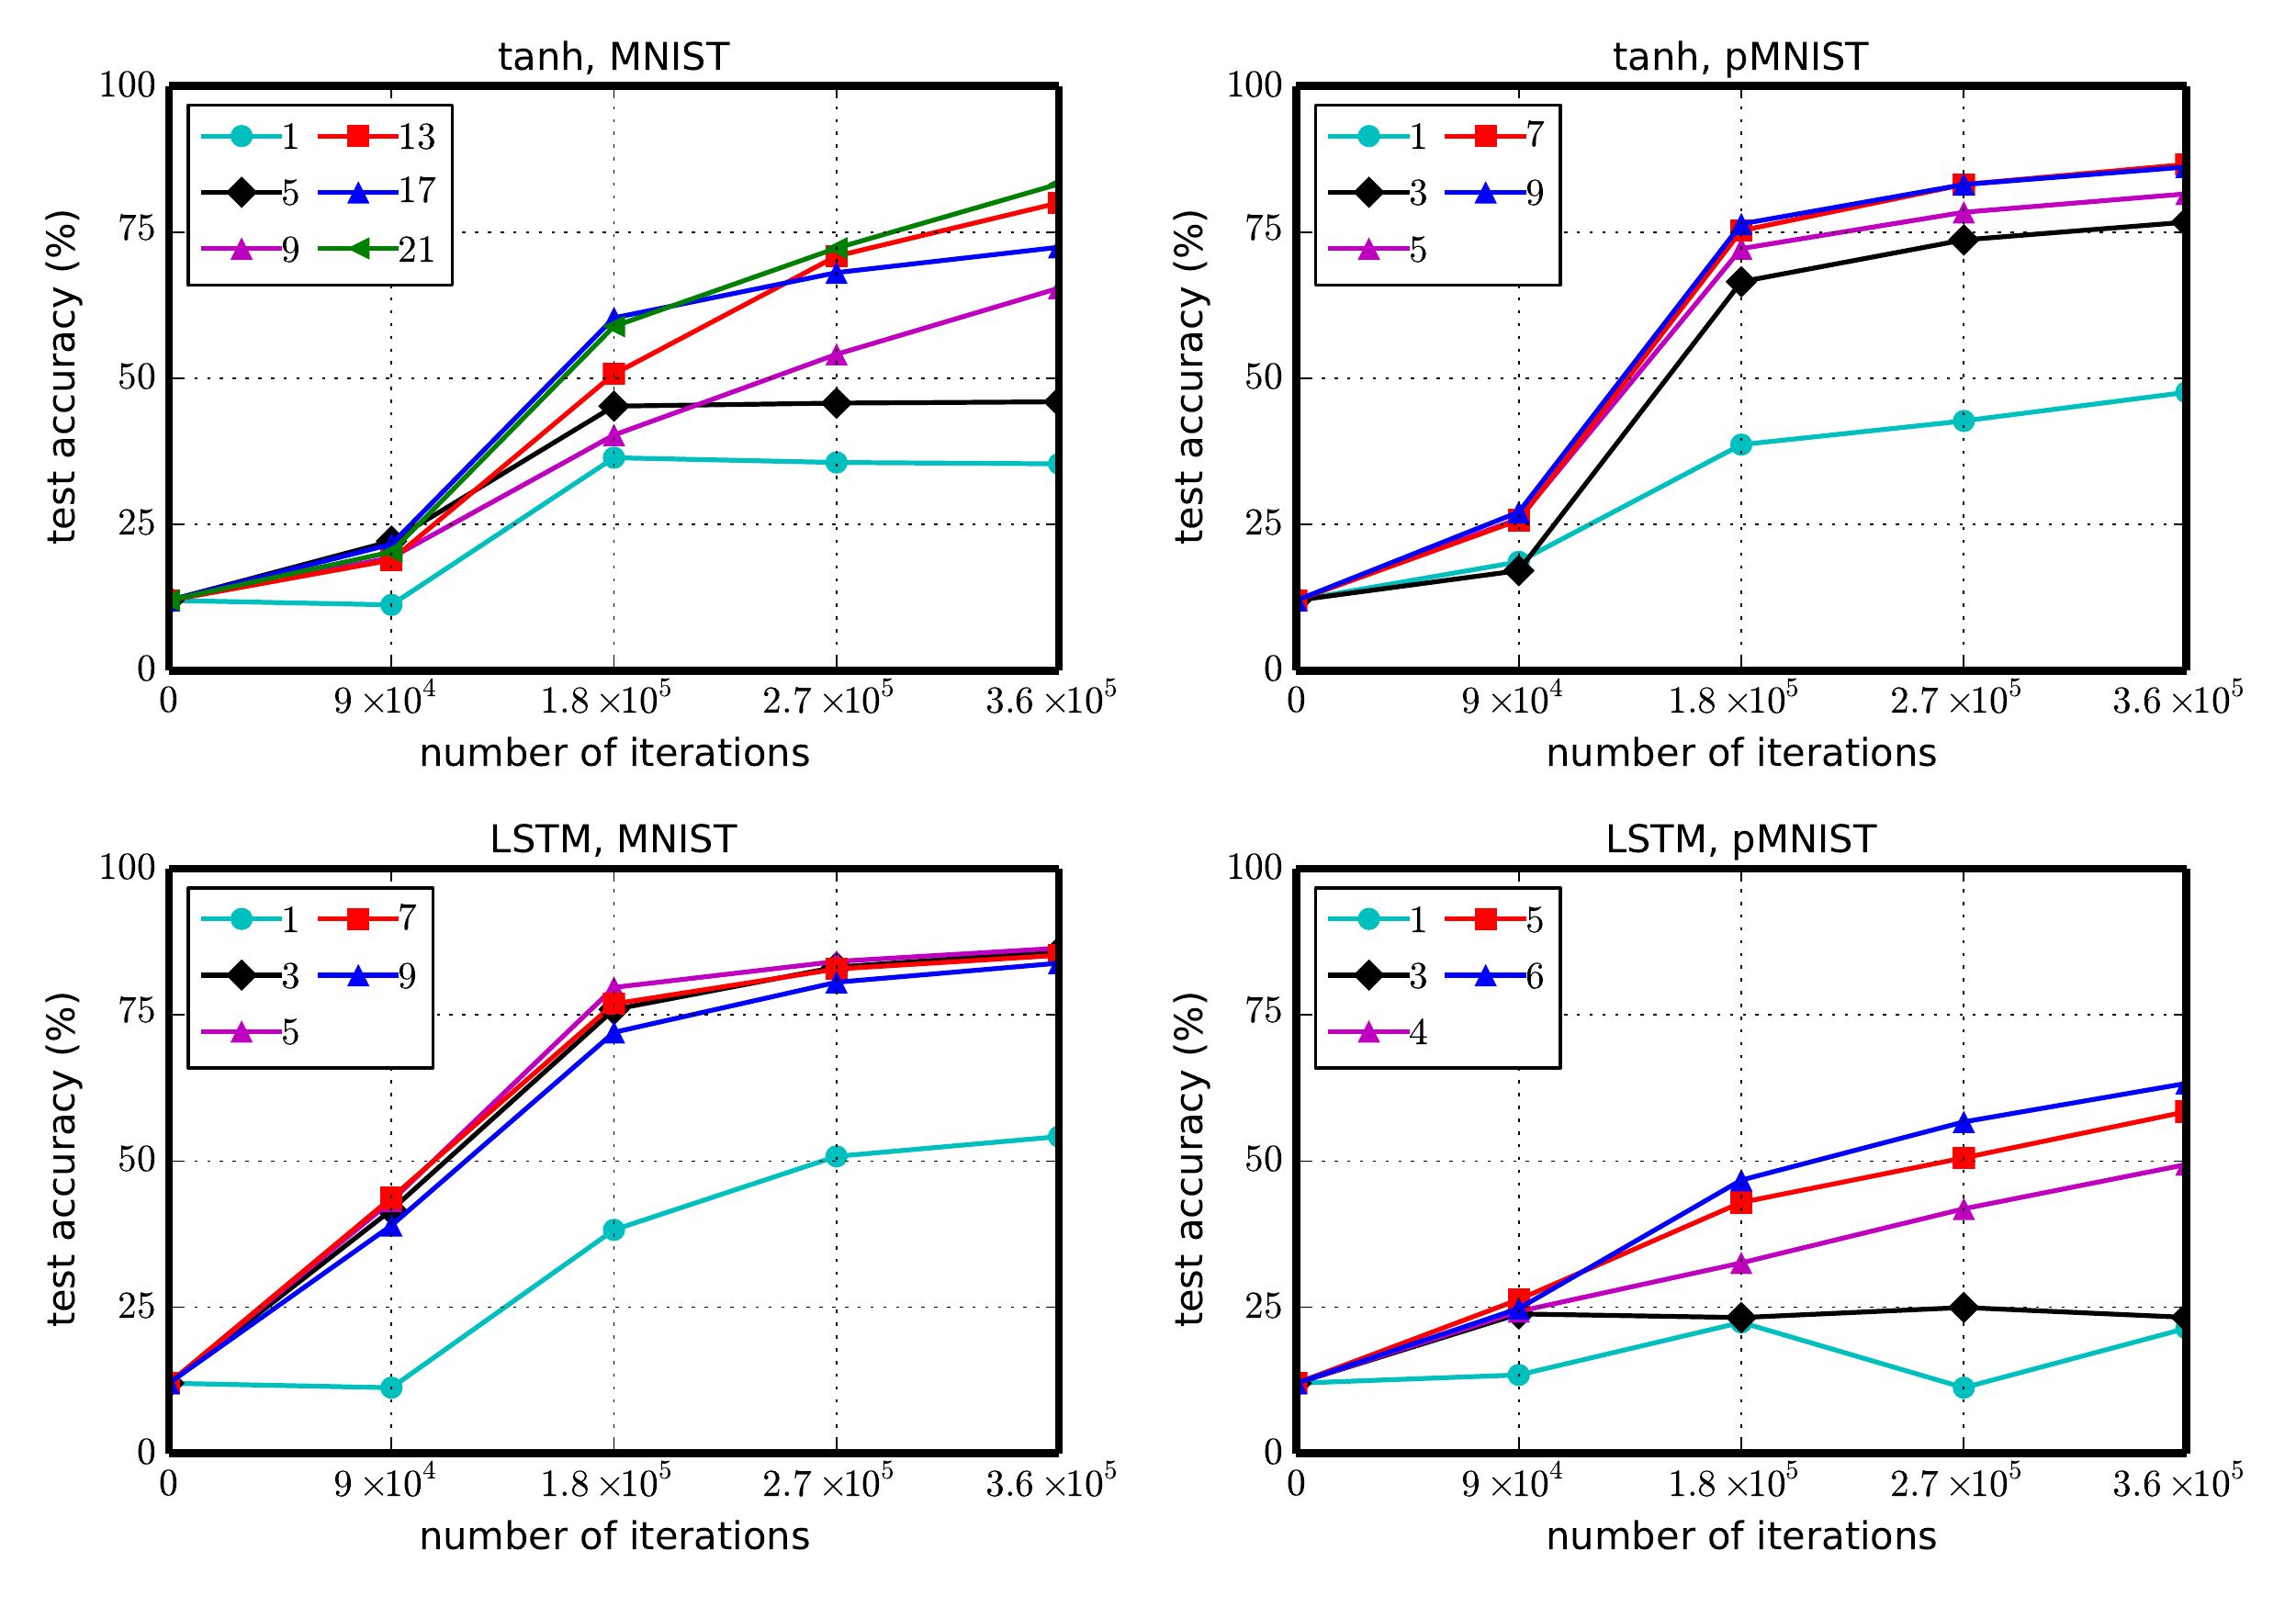}
\vspace{-10pt}
\caption{Test curves on MNIST/$p$MNIST, with $\tanh$ and $LSTM$. The numbers in the legend
denote the recurrent skip coefficient $s$ of each architecture.}
\label{fig:mnist_ex}
\end{figure}




\begin{figure}[htp]
\center
\includegraphics[width=350pt]{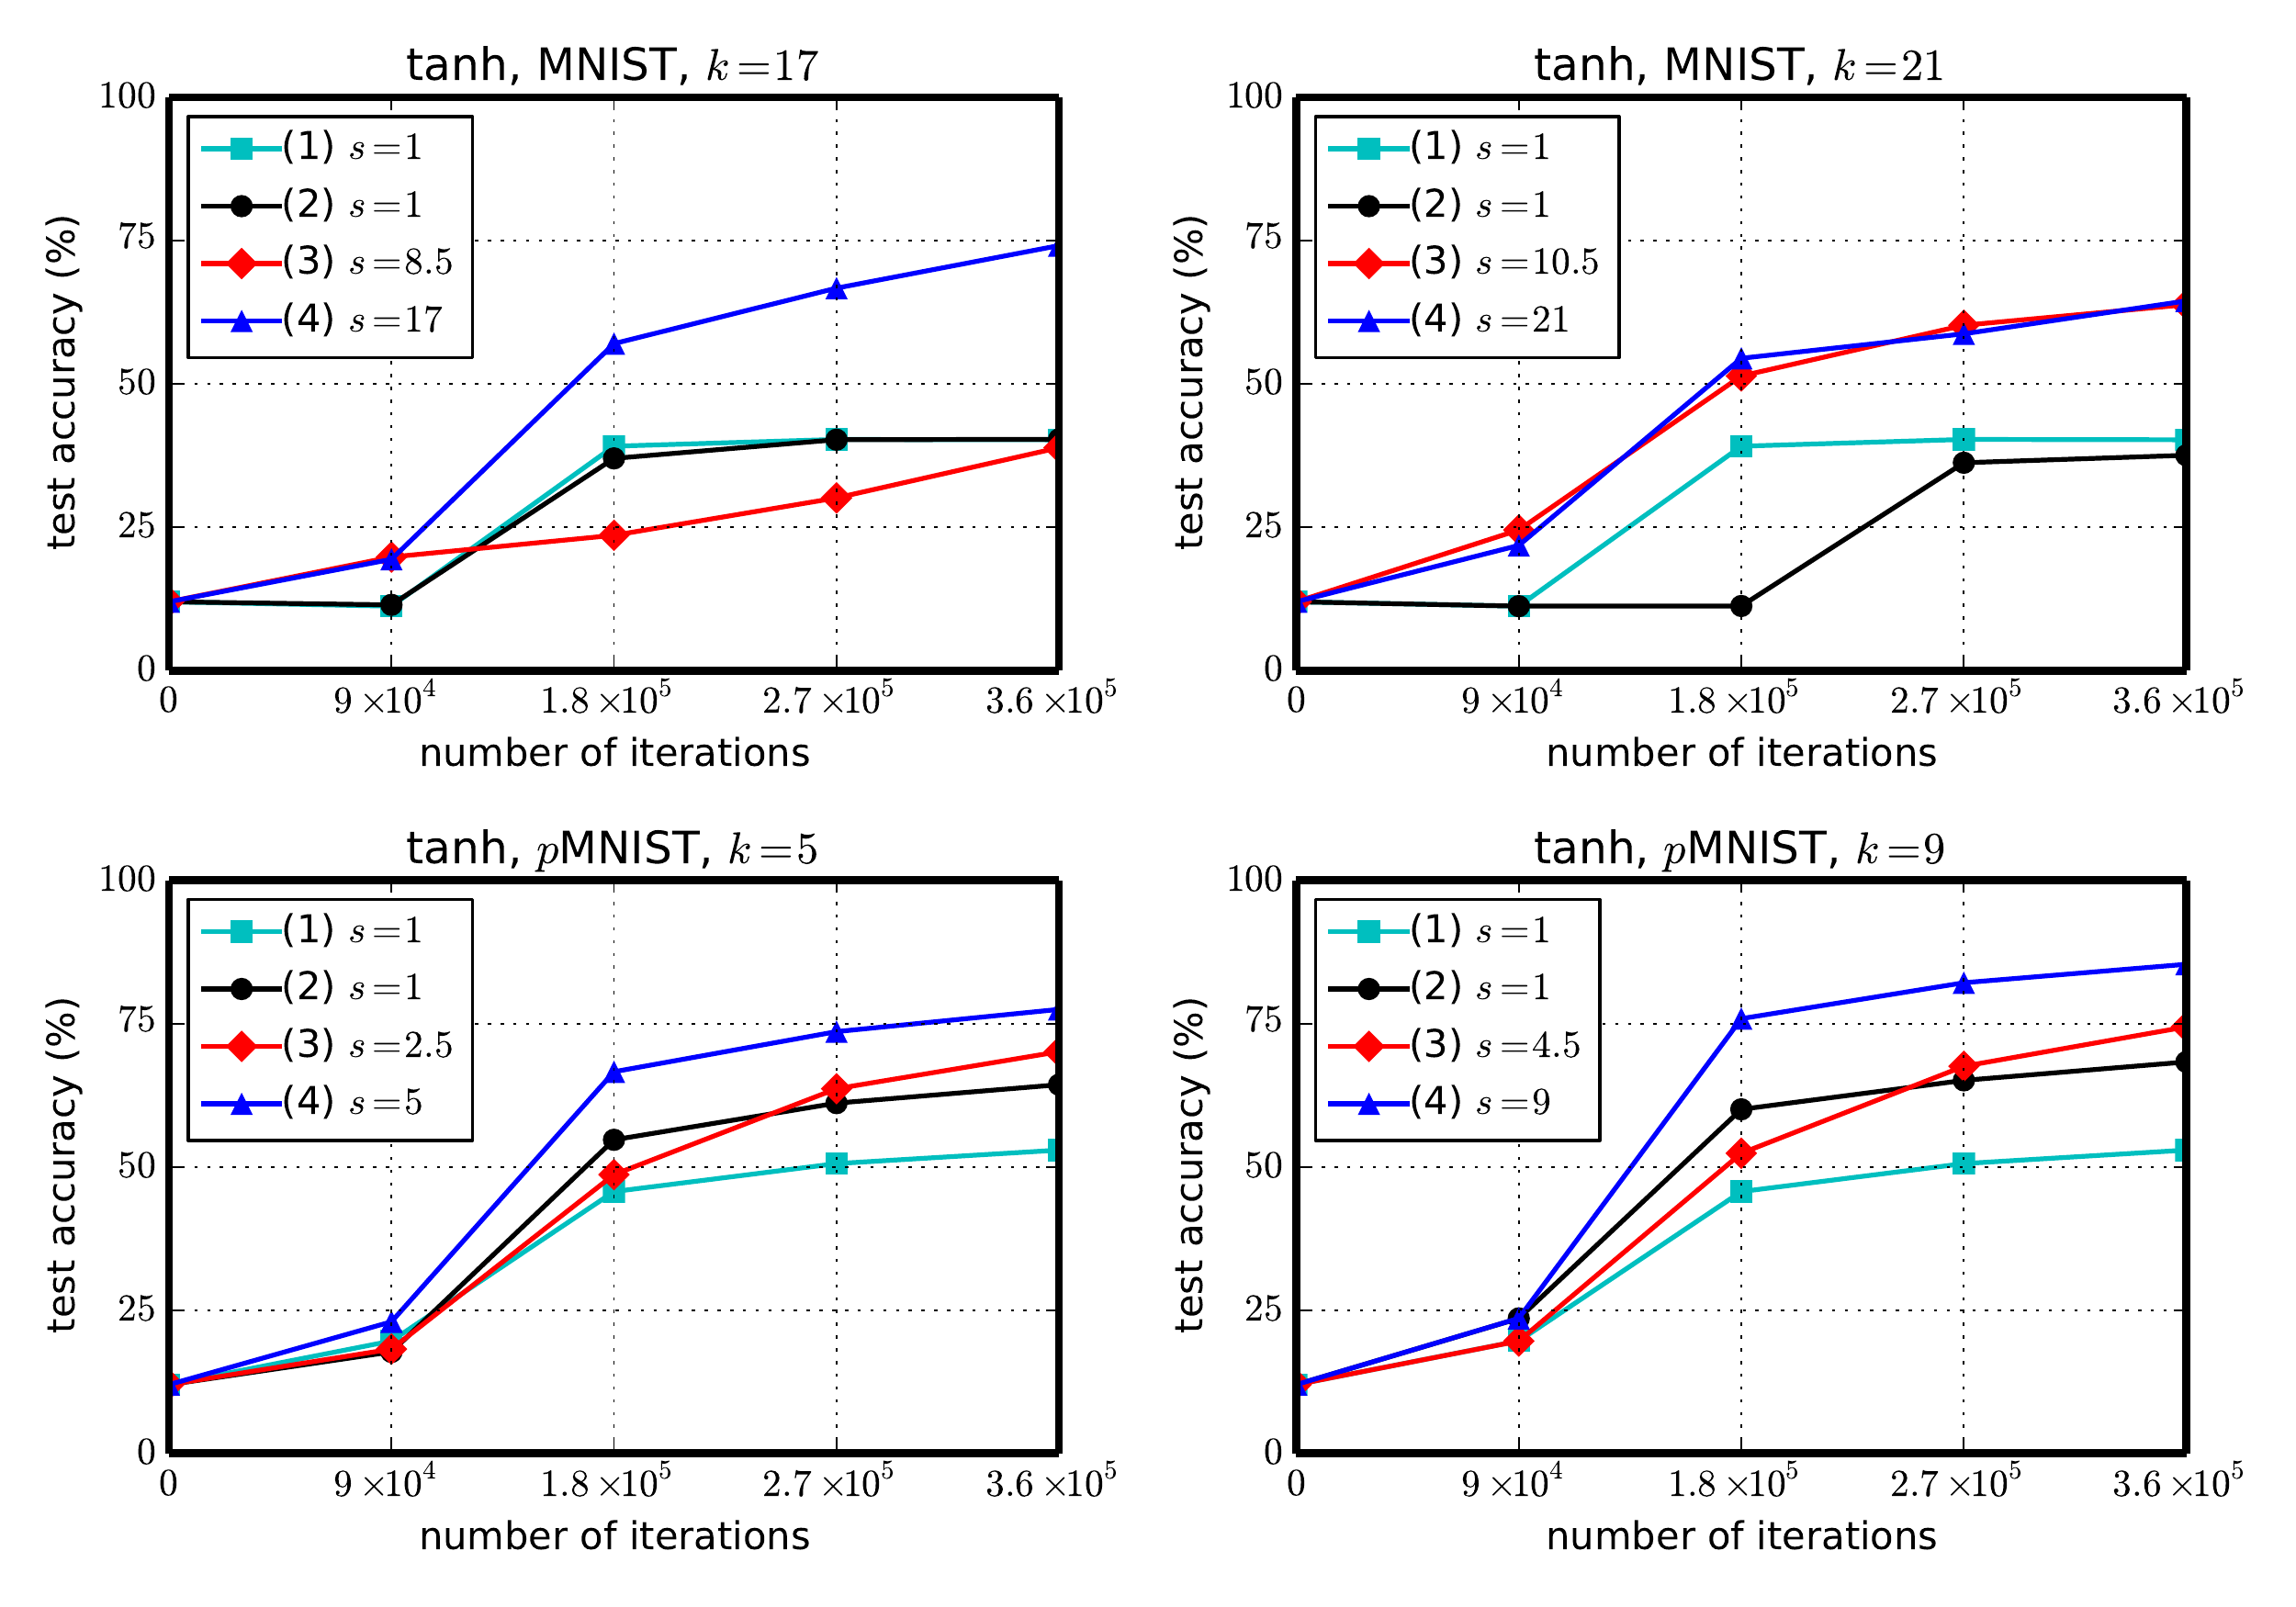}
\vspace{-10pt}
\caption{Test curves on MNIST/$p$MNIST for architecture (1), (2), (3) and (4), with $\tanh$.
The recurrent skip coefficient $s$ of each architecture is shown in the legend.}
\label{fig:verify_ex}
\end{figure}


%\section{miscellaneous}
% TODO: this sentence comes out strangely out of nowhere. What is ``this'' referring to?

{\small 
\bibliography{1recdepth}
\bibliographystyle{unsrt}
}
\appendix
%\end{document}


% This document was modified from the file originally made available by
% Pat Langley and Andrea Danyluk for ICML-2K. This version was
% created by Lise Getoor and Tobias Scheffer, it was slightly modified  
% from the 2010 version by Thorsten Joachims & Johannes Fuernkranz, 
% slightly modified from the 2009 version by Kiri Wagstaff and 
% Sam Roweis's 2008 version, which is slightly modified from 
% Prasad Tadepalli's 2007 version which is a lightly 
% changed version of the previous year's version by Andrew Moore, 
% which was in turn edited from those of Kristian Kersting and 
% Codrina Lauth. Alex Smola contributed to the algorithmic style files.  
